# Supplementary material for: Comparison between explicit and implicit discretization strategies for a dissipative thermal environment
Source: arXiv:2601.13103 source file (2026-01-19)
Supplement: Supplementary file 1 [file si.pdf]

# Supplementary Materials: Comparison Between Explicit and Implicit Discretization Strategies for a Dissipative Thermal Environment

Xinxian Chen[1] and Ignacio Franco[1, 2, 3, a)]

[1)] *Department of Chemistry, University of Rochester, Rochester, New York 14627, United States*

[2)] *Department of Physics and Astronomy, University of Rochester, Rochester, New York 14627, United States*

[3)] *The Institute of Optics, University of Rochester, Rochester, New York 14627, United States*

(Dated: 13 December 2025)

[a)] Electronic mail: ignacio.franco@rochester.edu

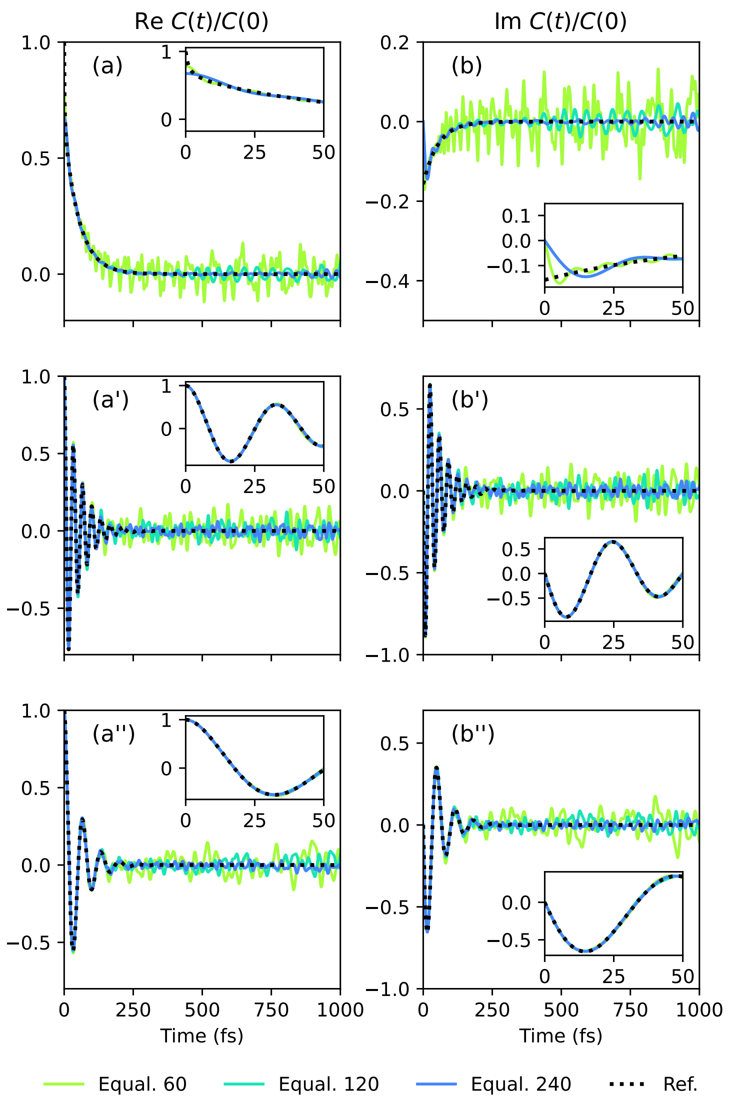


FIG. S1. Bath correlation function decomposition in the time domain using the equalized discretization with a cutoff frequency of 3000 cm$^{-1}$. (a) and (b): Drude–Lorentz with $\lambda_{\mathrm{D}}$ and $\gamma_{\mathrm{D}}$ to be the same as in Fig. 1; (a') and (b'): Brownian oscillator with $\lambda_{\mathrm{B}} = \lambda_{\mathrm{D}}$, $\gamma_{\mathrm{B}} = \gamma_{\mathrm{D}}$, and frequency $\omega_1 = 1000$ cm$^{-1}$; (a") and (b"): Brownian oscillator with $\lambda_{\mathrm{B}} = \lambda_{\mathrm{D}}$, $\gamma_{\mathrm{B}} = \gamma_{\mathrm{D}}$, and $\omega_1 = 500$ cm$^{-1}$.

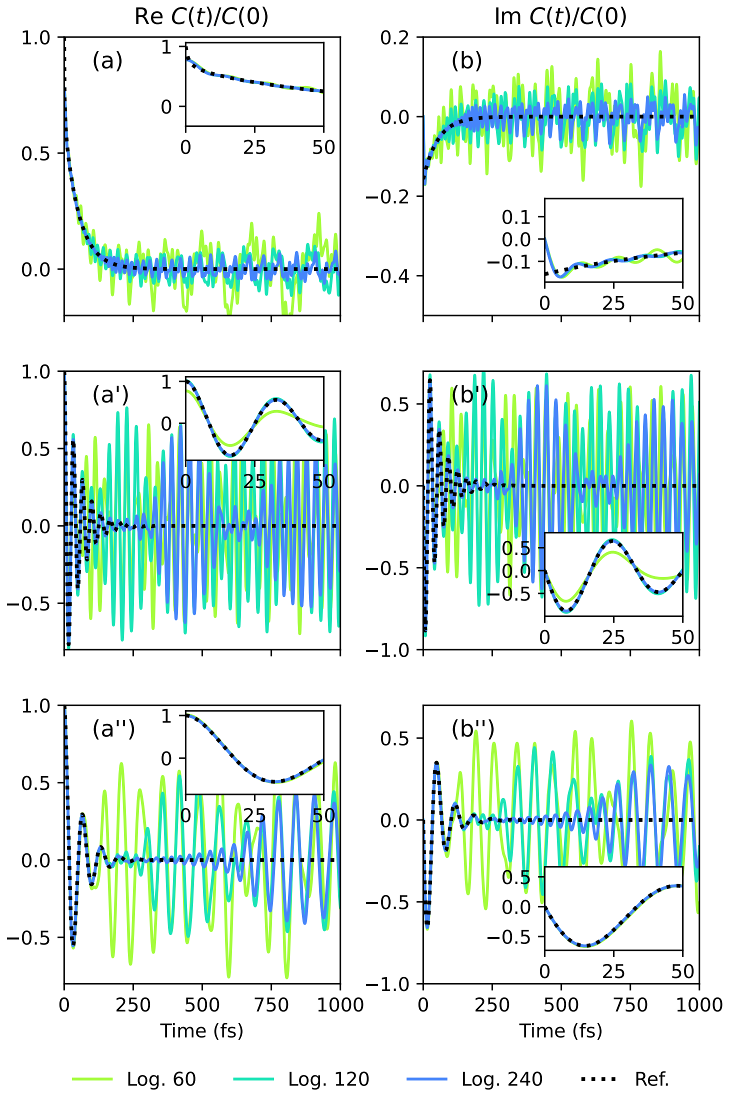


FIG. S2. Bath correlation function decomposition in the time domain as in Fig. S1 but using the logarithmic discretization.

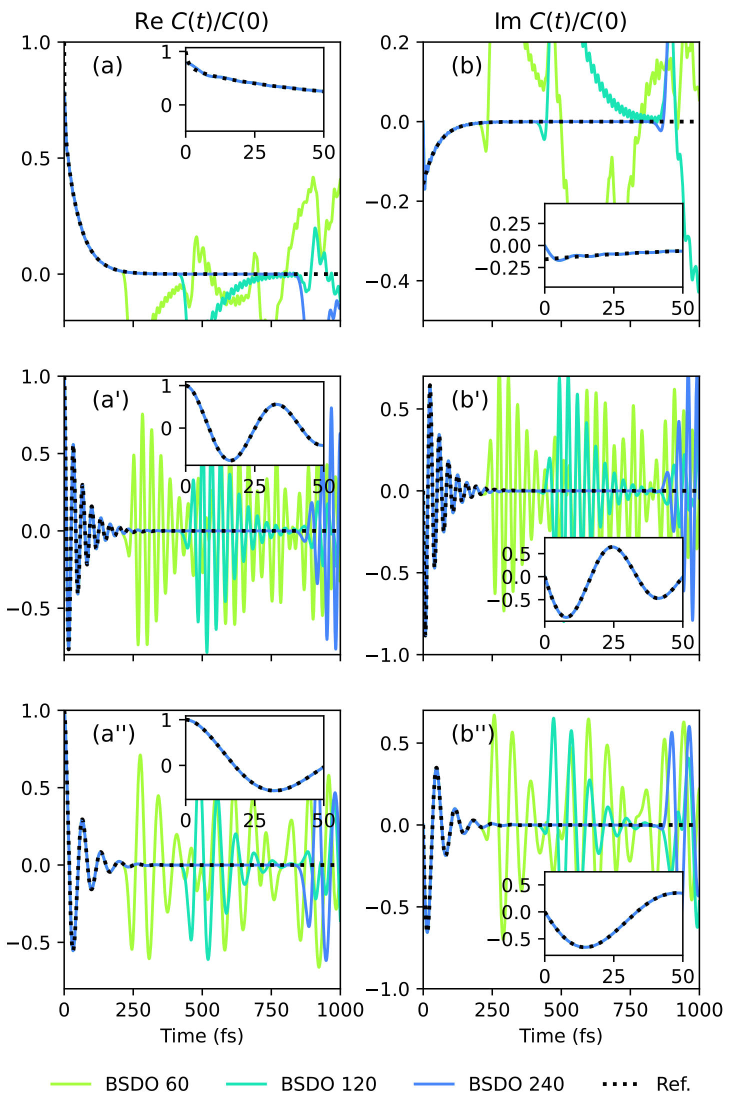


FIG. S3. Bath correlation function decomposition in the time domain as in Fig. S1 but using the BSDO discretization.

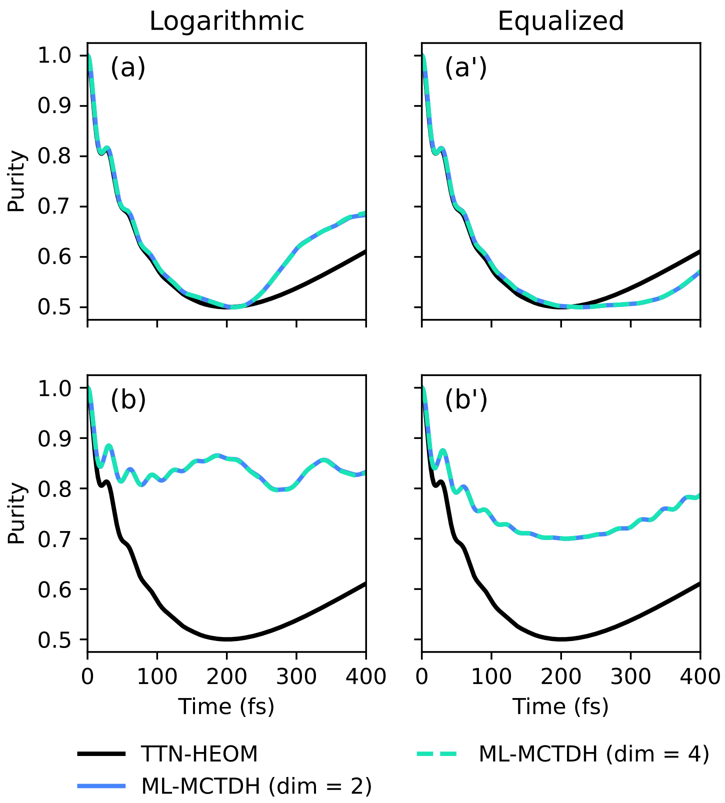


FIG. S4. Convergence of primitive basis dimensions for ML-MCTDH computation using logarithmic discretization [(a) and (b)] and equalized discretization [(a') and (b')] with 120 modes for the two-level system coupled to a Drude–Lorentz bath with a cutoff frequency 3000 $cm^{-1}$ [(a) and (a')] and 1000 $cm^{-1}$ [(b) and (b')]. The dimensions for each primitive basis are showed in the bracket in the labels. For 120 discretized mode, the primitive basis dimension of 2 can already reach the converged result with the dimension of 4 within the first 400 fs, where the same divergence emerges from the TTN-HEOM results for the thermalization dynamics.
